# Supplementary material for: Tunable reciprocal and nonreciprocal contributions to 1D Coulomb Drag
Source: arXiv:2408.12737 ancillary file (2026-03-23)
Supplement: Supplementary file 1 [file Supplemental_Material.pdf]

# Supplementary Materials: “Tunable Contributions from rectification and momentum transfer to 1D Coulomb Drag”

Mingyang Zheng,<sup>1</sup> Rebika Makaju,<sup>1</sup> Rasul Gazizulin,<sup>1,2</sup> Sadvikas J. Addamane,<sup>3</sup> and D. Laroche<sup>1,\*</sup>

<sup>1</sup>*Department of Physics, University of Florida, Gainesville, FL 32611, USA*

<sup>2</sup>*National High Magnetic Field Laboratory High B/T Facility,  
University of Florida, Gainesville, 32611, FL, USA*

<sup>3</sup>*Center for Integrated Nanotechnologies, Sandia National Laboratories, Albuquerque, NM 87185, USA*

## I. DEVICE FABRICATION

### A. Vertically-integrated double quantum wires

The vertically-integrated double quantum wires used in this article are patterned on an n-doped GaAs/AlGaAs electron bilayer heterostructure (wafer VA1110). The two 18 nm wide quantum wells are separated by a 15 nm wide  $\text{Al}_{0.3}\text{Ga}_{0.7}\text{As}$  barrier. The unpatterned density and mobility of the GaAs quantum well are  $2.98 \times 10^{11} \text{ cm}^{-2}$ ,  $\mu = 7.4 \times 10^4 \text{ cm}^2/\text{V} \cdot \text{s}$ , respectively. Two sets of two split gates are deposited using electron beam lithography on the upper and the lower side of the sample using an epoxy-bound-and-stop-etch (EBASE) process. These gates define two wires that are  $\sim 5 \mu\text{m}$  long and  $\sim 0.6 \mu\text{m}$  wide. More details on the fabrication process are presented elsewhere [1]. A microscopy image of the finished vertically-integrated quantum wires is presented in Fig. S1(a), along with a zoom-in microscopy image of the wire overlapping region in Fig. S1(b). In Fig. S1(b), the lower wire design is overlapped with the zoom-in microscopy image, demonstrating the good alignment between the two quantum wires.

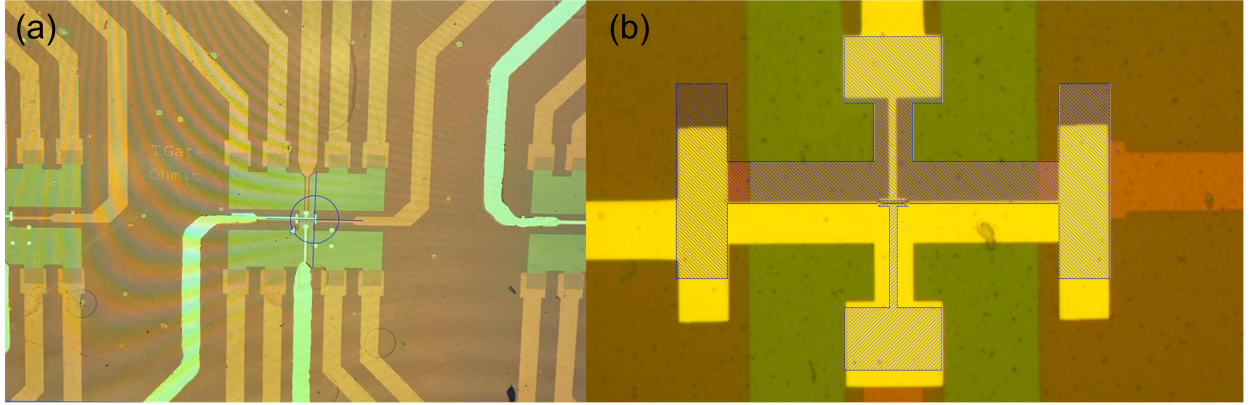

Fig. S1. Optical microscopy image and design of the vertical device. (a) Optical microscopy image of the vertical device. (b) Zoom-in image of the wire region. The wires overlapping region is shown. The lower wire design is overlapped with the zoom-in microscopy image.

### B. Laterally-integrated double quantum wires

A n-doped AlGaAs/GaAs heterostructure (VA182) with the 2DEG buried 80 nm below the surface is used as a starting point to fabricate the laterally coupled quantum wires. A mesa structure is patterned using standard photolithography techniques and defined using a wet phosphoric acid etch. Ohmic contacts (Ge/Au/Ni/Au of thickness

---

\* Email of Author to whom correspondence should be addressed: dlaroc10@ufl.edu

260 Å/ 540 Å/ 140 Å/ 960 Å) are then defined using photolithography and evaporated into the heterostructure, followed by an annealing step at 420°C for 1 min in a rapid thermal annealer. Finally, e-beam lithography is utilized to define the electrostatic gates (Ti-Au of thickness 100 Å- 1000 Å), which are deposited using sputtering. The quantum wires in the device are separated by  $\sim 150$  nm. An optical microscopy image of a typical device with the gates and the ohmic contacts is shown in Fig. S2(a), along with a scanning electron microscope image in Fig. S2(b). The device is defined by three gates, allowing for independent contacts to each quantum wire.

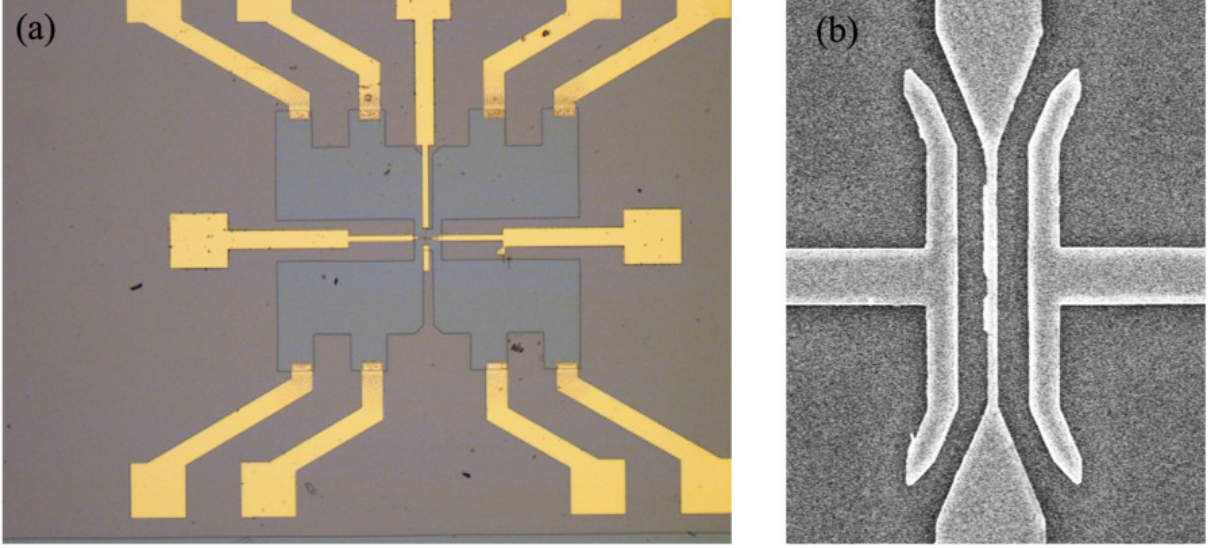

Fig. S2. Microscopy images of the lateral device. (a) Optical microscopy image of the lateral device. (b) Scanning electron microscope image of the wire region.

## II. ADDITIONAL DEVICE CHARACTERIZATION

A circuit diagram of the Coulomb drag measurement scheme utilizing a virtual ground on the drag side is presented in Fig. S3, where the drive current is applied on the top wire and the drag voltage is measured on the bottom wire. This setup ensures that no accidental bias is applied to the drag wire throughout the measurement. To prevent current flow from the drive wire to the drag wire, it is verified that tunneling between the two layers is negligible. The tunneling measurements are performed by sending a small source-drain voltage across the device for different top PO gate and bottom PO gate values, and then taking the numerical derivative of the resulting signal. Both top PO gate and bottom PO gate values were selected such that the tunneling resistance between the two wires was larger than  $10M\Omega$  in a bias range of  $\pm 1.5\text{mV}$ . Two examples of tunneling measurement are shown in Fig. S4. Fig. S4(a) and Fig. S4(b) show the tunneling conductance across the two layers when the top PO gate is at  $-0.39\text{V}$  and  $-0.43\text{V}$  respectively. The tunneling conductance is higher than  $10M\Omega$  when the top PO gate is at  $-0.43\text{V}$  and the bottom PO gate is below  $-0.36\text{V}$ .

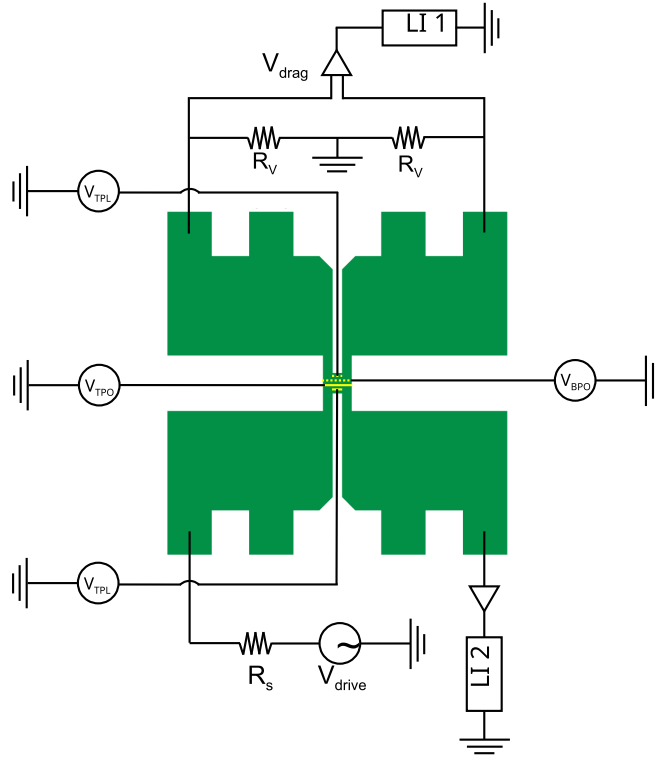

Fig. S3. Measurement setup. Circuit diagram for Coulomb drag measurements. A drive current is supplied to the top of the device and the drag voltage is measured in the bottom wire. The drive current is sourced using a  $R_s = 10\text{M}\Omega$  resistor in series with the drive wire. A virtual ground setup is used on the drag side of the experiment. Additionally, source-measure units are used to source and measure DC signals applied to the electrostatic gates.

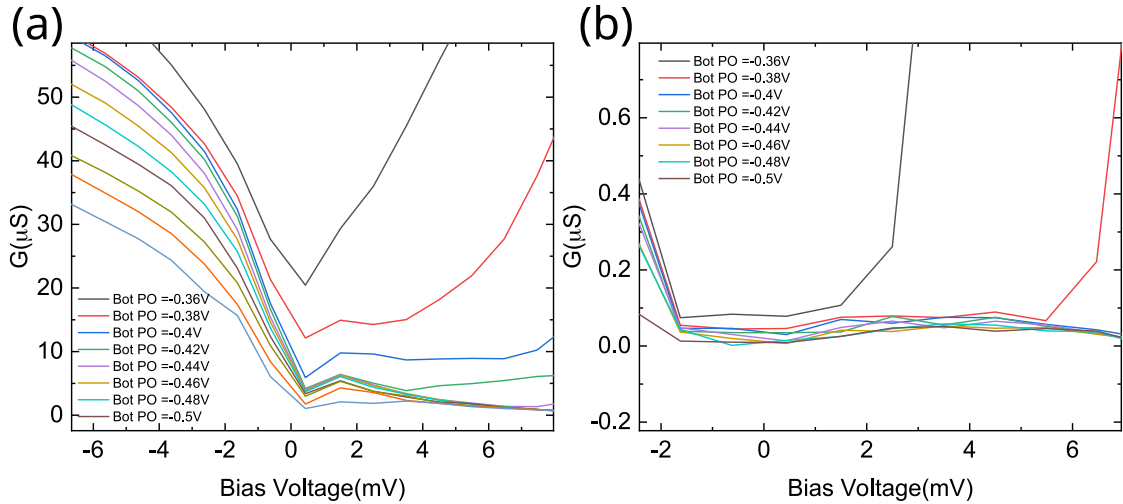

Fig. S4. Example of a 2D-2D tunneling measurement. The tunneling conductance is plotted against the source-drain bias across the tunnel barrier for various PO gate voltages. (a) The top PO gate at  $-0.39\text{V}$ , and (b) The top PO gate at  $-0.43\text{V}$ . The lines from top to bottom correspond to the bottom PO gate from  $-0.36\text{V}$  to  $-0.5\text{V}$  by  $-0.02\text{V}$  increments.

### III. ONSAGER'S RELATION

Onsager's relations have been used as an important verification of the dominance of momentum transfer component in the Coulomb drag measurements [1?–4]. However, the Onsager's relation is broken with the existence of charge rectification component [5–8]. In Fig. S5, we present the Onsager's relation tests by changing the direction of the drive current and exchanging the drive and drag wires at the base temperature of the cryostat in a liquid He<sub>3</sub> immersion cell. In Fig. S5(a) and Fig. S5(c), Onsager's relation is not obeyed when the drag and the drive wires are exchanged as the signals are not identical. With the drive current direction changed, the sign of the drag signal was reversed in some regions while other regions remained the same, confirming the existence of both momentum transfer and charge rectification components in the vertically-integrated double quantum wires.

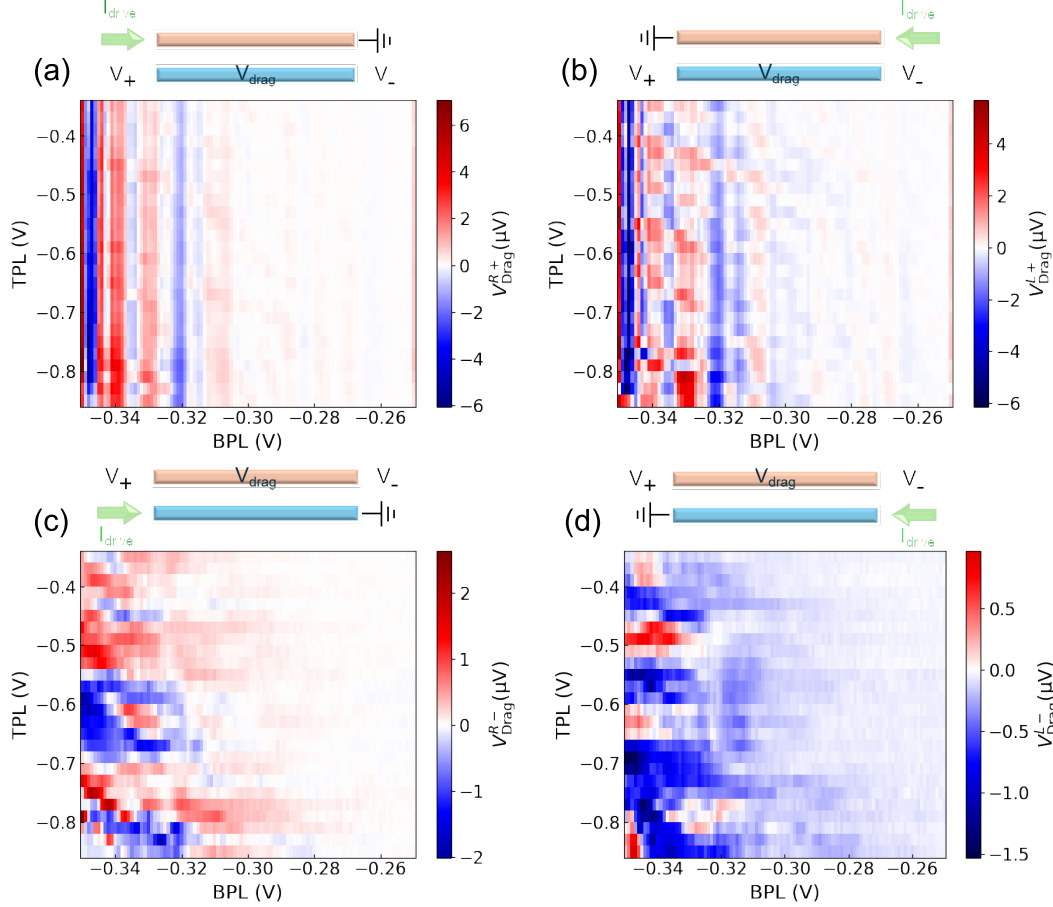

Fig. S5. Onsager's relations of the drag signal. The drag voltage is plotted as a function of both top PL and bottom PL gate voltages for various measurement configurations. (a) The top wire is used as the drive wire while the bottom wire is used as the drive wire. (b) same as (a), while the drive current direction is reversed. Onsager's relation is not obeyed as the signal's polarity remains virtually unchanged over large subsections of the experimental phase-space. (c) The top wire is used as the drag wire while the bottom wire is used as the drive wire. Onsager's relation is broken yet again when the drag and the drive wires are exchanged as the signals are not identical. (d) same as (c), while the drive current direction is reversed.

### IV. SUBBAND POSITIONS AND DRAG SIGN CHANGE

As shown in Fig. S6(a), the small conductance plateaus can be seen in the bottom wire scan at different BPL gate positions while their positions remain almost unchanged by changing the TPL gate value. In Fig. S6(b), each plateau corresponds to each local minimum in the first derivative of the bottom wire conductance. The red stripes overlapping with the local minimums represent different possible subbands. In the momentum transfer model, the drag signal depends strongly on the subband matching and will be enhanced at the opening of each subband. As shown in Fig. S6(c) and Fig. S6(d), in the low-temperature regime, the sign change positions of the symmetric component overlap

consistently with the drag wire subband positions while the antisymmetric component is primarily positive, with only a few regions with negative polarity for the drag voltage with no clear correlation to the 1D wire subbands positions. This different dependence on the drag wire subband also indicates the different mechanisms between momentum transfer and charge rectification which require additional theoretical work.

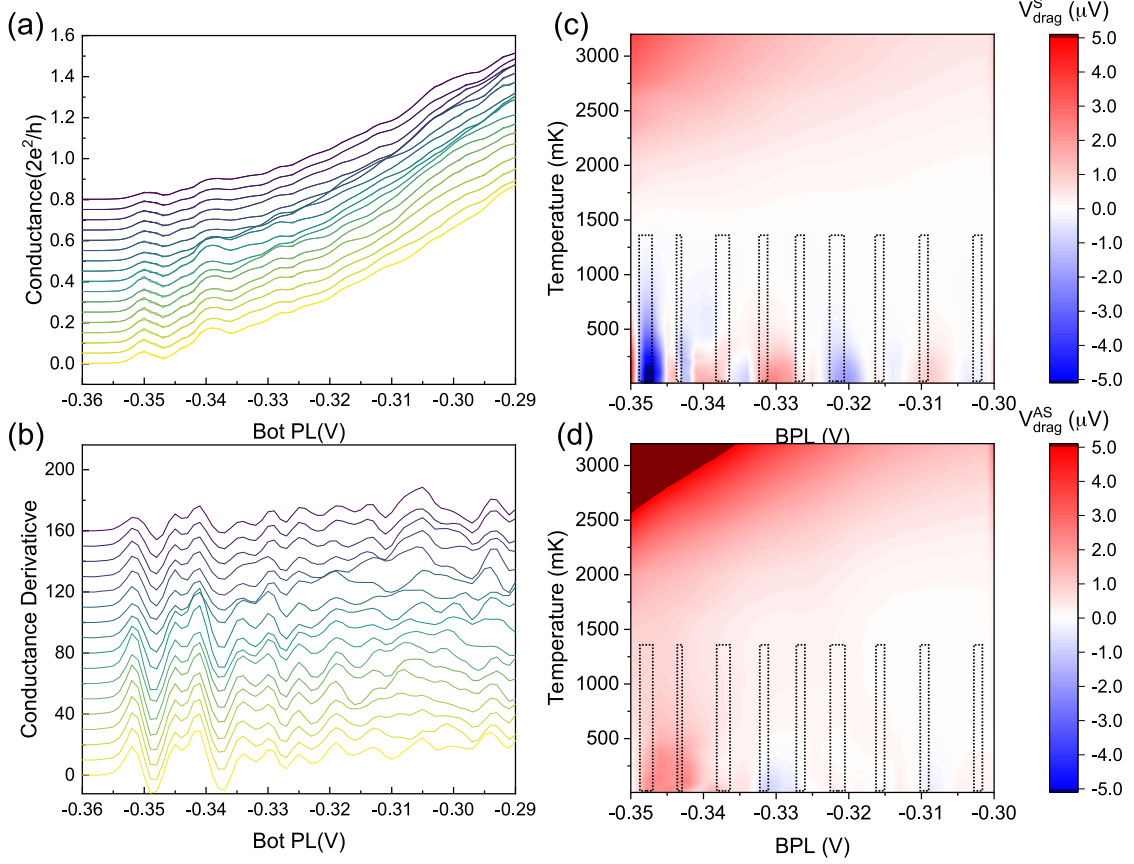

Fig. S6. Bottom wire subband positions and drag sign change. (a) Bottom (drag) wire conductance as a function of the bottom (drag) and top (drive) gate voltages. Interwire crosstalk is negligible compared to the top (drive) wire. Successive line-cuts are vertically offset by 0.05 ( $2e^2/h$ ) for visibility purposes. The top PL gate voltage ranges from -0.5V to -0.82V from bottom to top. (b) The first derivative of the smoothed data in (a). The red vertical stripes overlap with the local minimum of the conductance derivative, which corresponds to the possible bottom wire 1D subbands. (c), (d), BPL gate-temperature 2D plot at TPL=-0.735V of (c) the symmetric component and (d) the antisymmetric component. The dotted boxes correspond to the bottom(drag) wire subband positions.

## V. GATE AND TEMPERATURE TUNABLE RECTIFIED DRAG

Similarly to Fig. 3 in the main text, the BPL gate-temperature tunable rectified drag 2D maps for two other line cuts at TPL=-0.5475V and TPL=-0.6225V are shown in Fig. S7. Two distinct temperature regimes can still be identified in this data: a low-temperature regime below  $\sim 1.5$ K where both components exhibit BPL gate-tunable sign changes in the drag voltage polarity and a high-temperature regime where the drag signal is strictly positive, increases with increasing temperature and is dominated by the antisymmetric component. Similar to the  $r_{SAS}$  shown in Fig. 2 at base temperature, the  $r_{SAS}$  at 100mK is shown in Fig. S8. The results are similar to those taken at base temperature, with only a slight decrease in the range of the symmetric component's dominant region.

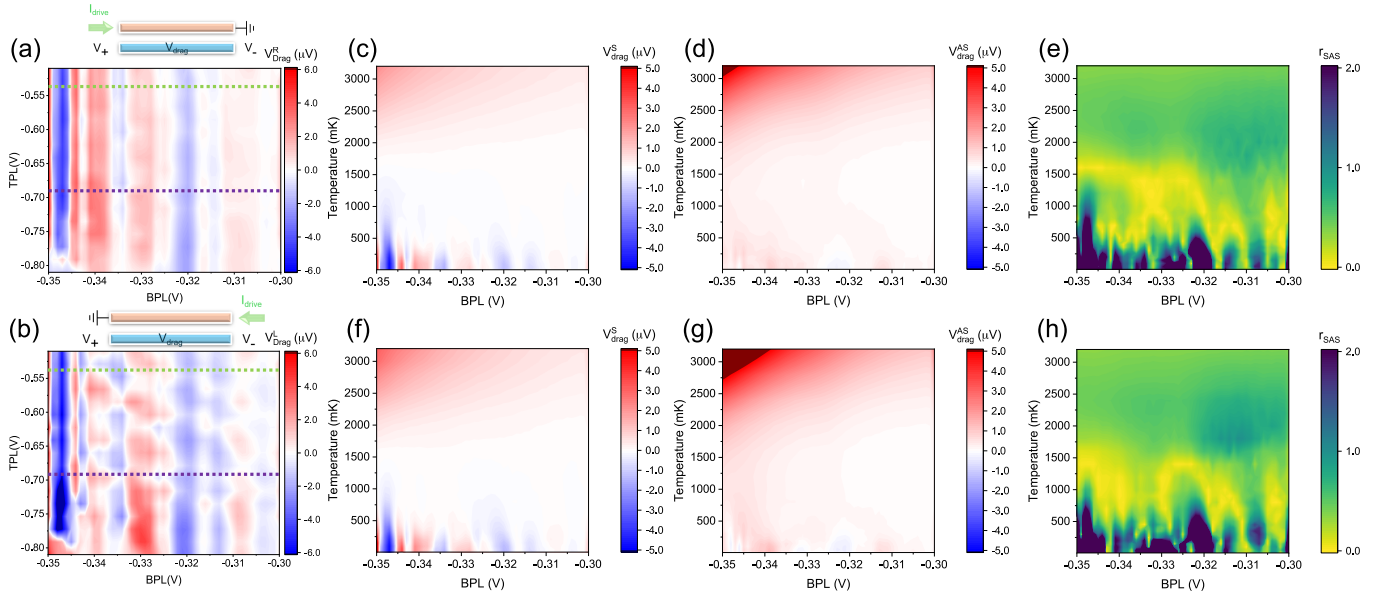

Fig. S7. Gate and Temperature tunable rectified drag. (a), (b) Drag map of the vertically-coupled device. (a) Drag voltage as a function of the top (drive) and bottom (drag) gate voltages when the drive current is in the same direction as the drag voltage measurement. (b), same as (a), with the drive current direction reversed. (c), (d), (e), BPL gate-temperature 2D plot at  $TPL = -0.5475V$  of (c) the symmetric component, (d) the antisymmetric component and (e)  $r_{SAS}$ . (f), (g), (h), BPL gate-temperature 2D plot at  $TPL = -0.6788V$  of (f) the symmetric component, (g) the antisymmetric component and (h)  $r_{SAS}$ .

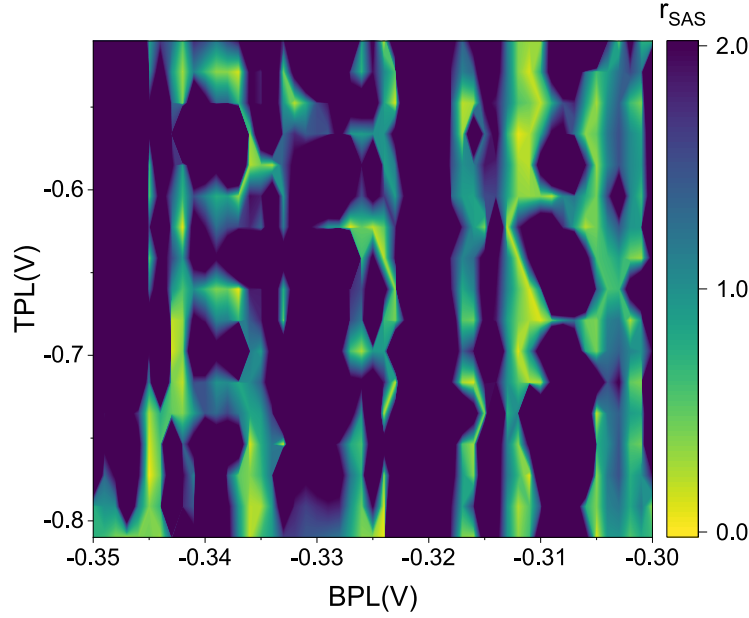

Fig. S8. Rectified drag at 100 mK. The  $r_{SAS}$  as a function of the top (drive) and bottom (drag) gate voltages at 100 mK.

## VI. CALCULATION OF THE ERROR BARS OF THE POWER-LAW AND ARRHENIUS FITTING

As shown in Fig. S9,  $V_{drag}^S$  and  $V_{drag}^{AS}$  both have linear regimes in the high-temperature part of a log-log plot. However, the range of linearity is different for different gate positions and different components. To fit the linear part, a starting range of  $N$  and an error limit  $E$  are initially chosen. Once the fitting slope  $S_N$  and intercept  $I_N$  of the starting range are calculated, a new point is added to the range, and a new fitting is performed, with slope  $S_{N+1}$  and intercept  $I_{N+1}$ . If  $\frac{|S_N - S_{N+1}|}{S_N} < E$ , this fitting range is increased further, otherwise, the range  $N$  is the set, and  $S_N$  and  $I_N$  are the final fitting parameters. The final error of the slope and the intercept is determined to be  $|S_N - S_{N+1}|$  and  $|I_N - I_{N+1}|$ , respectively. As shown in Fig. S9(d) and Fig. S9(h), the first few points are linearly fitted well while the slope will gradually change as the fitting range gets larger, once the change of fitting slope exceeds the error limit  $E$ , fitting will stop. Changing the  $N$  and  $E$  allows both power-law and Arrhenius data to be reliably fitted.

In the low-temperature regime, the fitting procedure is similar. A key difference is that the fitting range expands in both direction rather than in a single one. After reaching the error limit, the fitting will stop. Fig. S10 shows some low-temperature power-law and Arrhenius fitting results. The data points with “poor fitting” or sign changes were omitted. Although some trends of exponent decreasing within each subband are consistent with Fig. 5(c), the data appears too noisy to extract useful information, and are simply included here for completeness. The exception of S10d, where the data is comparable to the one presented in Fig. 5(b). Fig. S11 shows a few examples of the “poor fittings” mentioned previously, and are compared with some “good fitting” examples.

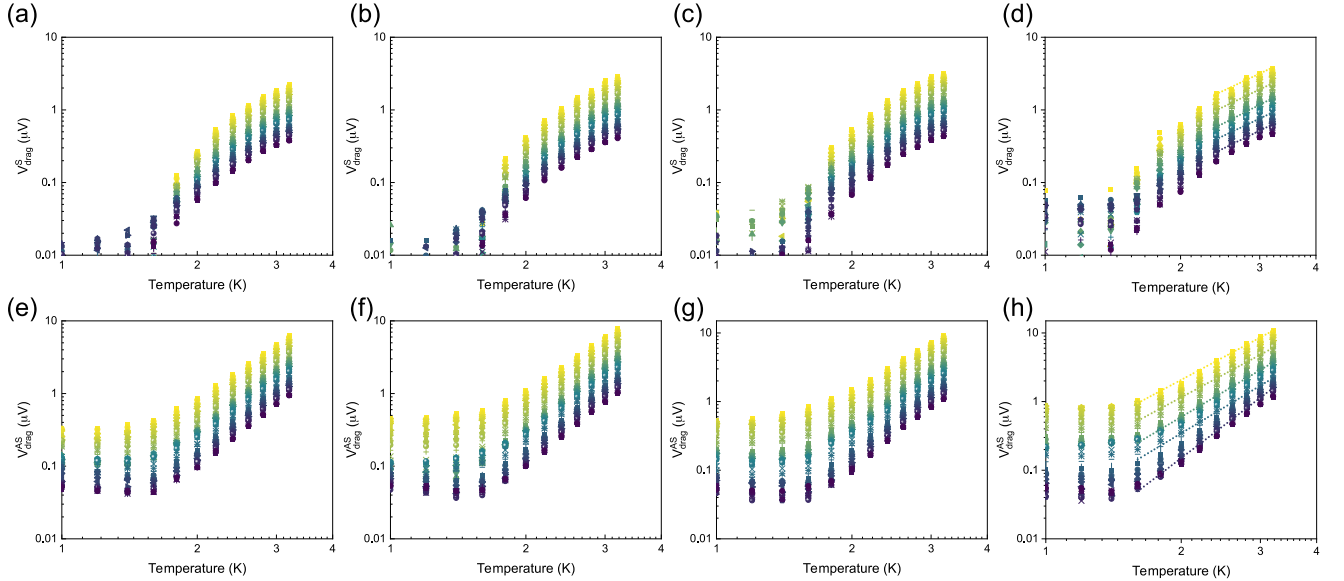

Fig. S9. All line cuts for selecting the power-law exponent in the high-temperature regime. (a), (b), (c), (d), The temperature dependent  $V_{drag}^S$  for four line cuts from 1K to 3.2K (a) TPL=-0.5475V, (b) TPL=-0.6225V, (c) TPL=-0.6788V and (d) TPL=-0.735V. (e), (f), (g), (h), The temperature dependent  $V_{drag}^{AS}$  for four line cuts from 1K to 3.2K (e) TPL=-0.5475V, (f) TPL=-0.6225V, (g) TPL=-0.6788V and (h) TPL=-0.735V. The BPL gate voltage ranges from -0.35V to -0.301V from top to bottom in each line cut with color changes from yellow to blue. The dotted lines are linear fitting examples. The amplitude changes with BPL gate voltage agree with the stronger drag signal at lower electron density in the wires. The linear ranges of the antisymmetric components in the log-log plot are larger than that of the symmetric components.

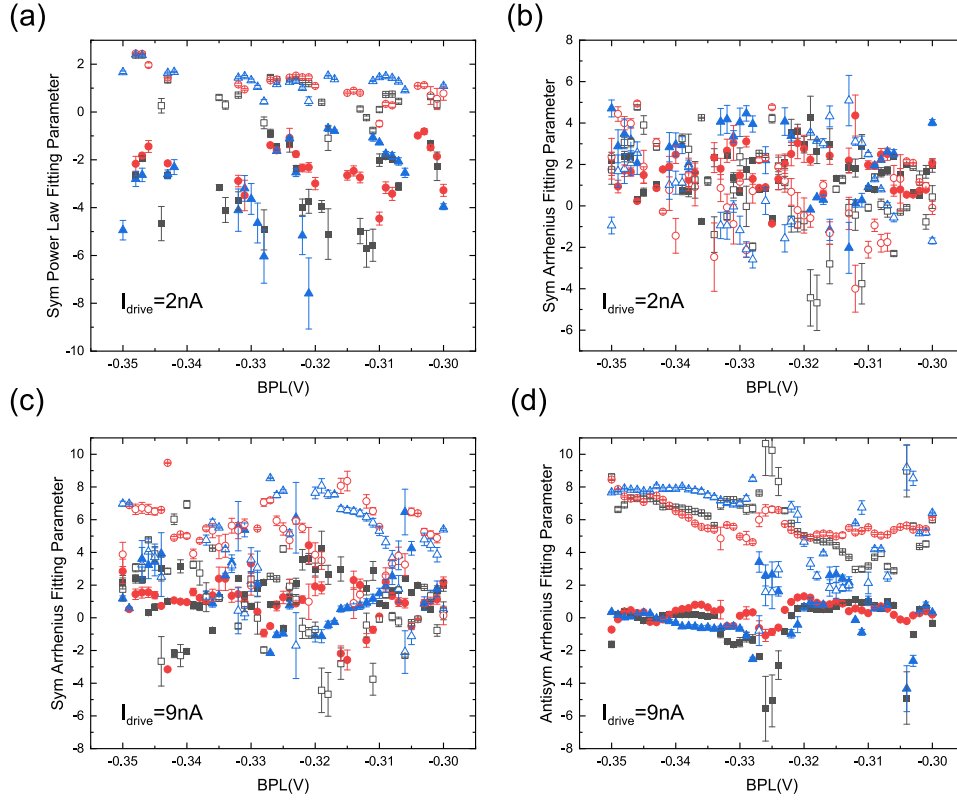

Fig. S10. Low-temperature regime line cut analysis. Extracted power-law and Arrhenius in fitting parameters include power-law exponent (solid symbols) and magnitude (open symbols) in the temperature range 0.1K to 1.4K for TPL=-0.735V (black circles), TPL=-0.6225V (red squares), and TPL=-0.5475V (blue triangles). (a) Power-law fitting results of the symmetric component when the drive current is 2nA. (b) Arrhenius fitting results of the symmetric component when the drive current is 2nA. (c) Symmetric component Arrhenius fitting results when the drive current is 9nA. (d) Antisymmetric component Arrhenius fitting results when the drive current is 9nA.

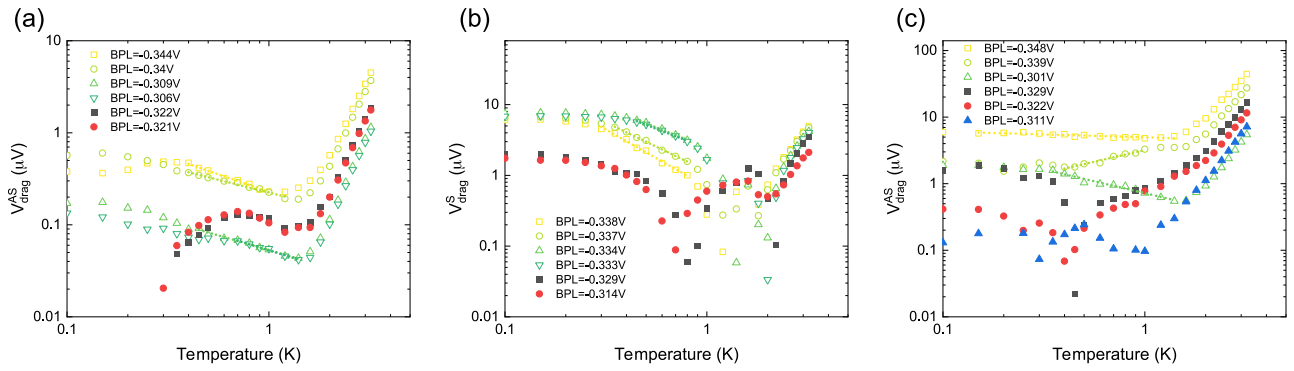

Fig. S11. Low-temperature range line cut “poor fitting” examples. The temperature dependent  $V_{drag}^S$  and  $V_{drag}^{AS}$  “poor fitting” examples for Fig. 5 include “poor fitting” points (solid) and “good fitting” points (open) in the temperature range 0.1K to 1.4K. (a) Power-law fitting results of the antisymmetric component when the drive current is 2nA at TPL=-0.5475V. (b) Symmetric component power-law fitting results when the drive current is 9nA at TPL=-0.6225V. (c) Antisymmetric component power-law fitting results when the drive current is 9nA at TPL=-0.735V. The dotted lines are examples of the linear fitting lines for the “good fitting” points in the log-log plot.

## VII. HIGH-TEMPERATURE LINE CUT ARRHENIUS FITTING

Besides the power-law fitting of the high-temperature line cut of the symmetric and antisymmetric components, Arrhenius fittings were also done to compare with prospective theoretical candidates. These fittings are shown in Fig. S12. For all selected line cuts, the Arrhenius magnitude has a monotonous decrease with increasing drag wire electron density, which is consistent with the power-law fitting results in Fig. 4. However, compared to the power-law exponents' dependence on the drag wire subband changes, the Arrhenius exponents show no obvious oscillation with the drag wire electron density, which is against the theoretical predictions, and is thus not considered likely to reflect our data.

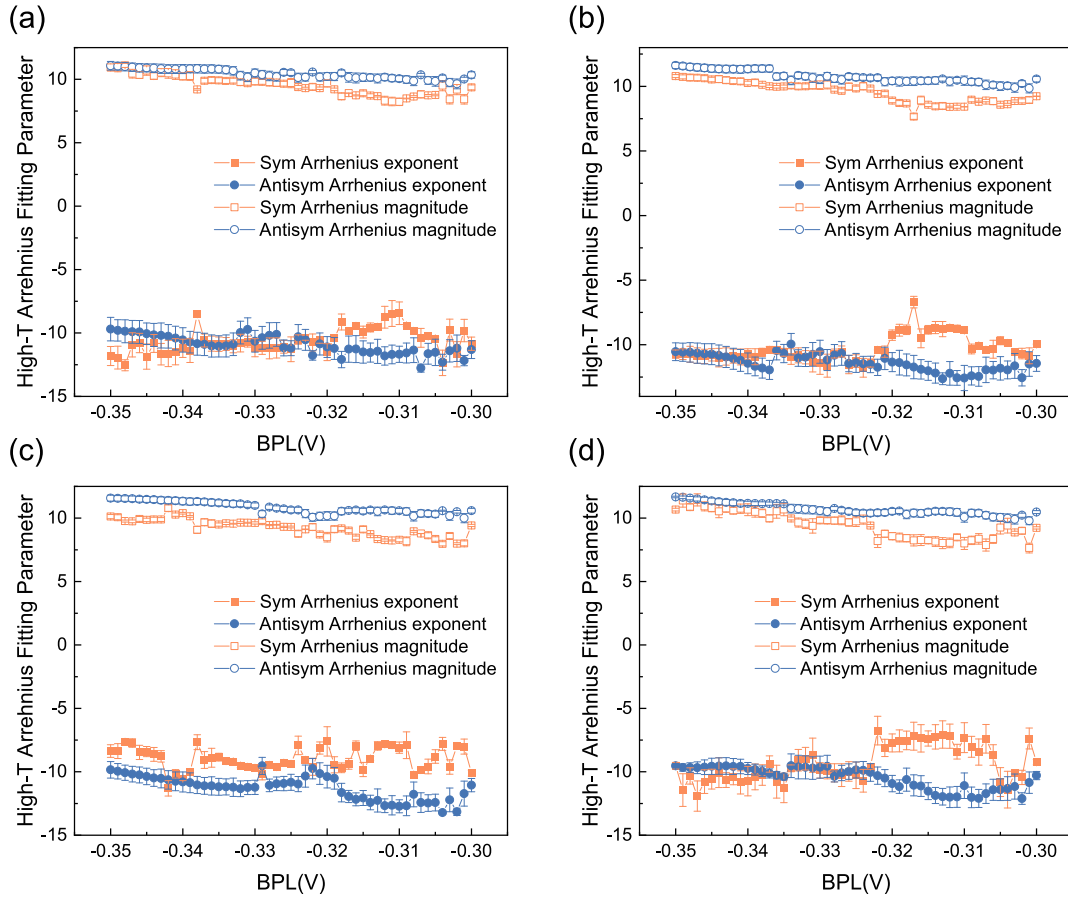

Fig. S12. High-temperature line cut Arrhenius fitting. Extracted Arrhenius fitting parameters include exponent (solid symbols) and magnitude (open symbols) for (a) TPL=-0.5475V, (b) TPL=-0.6225V, (c) TPL=-0.6788V and (d) TPL=-0.735V. Both the symmetric component (orange) and the antisymmetric (blue) components are presented.

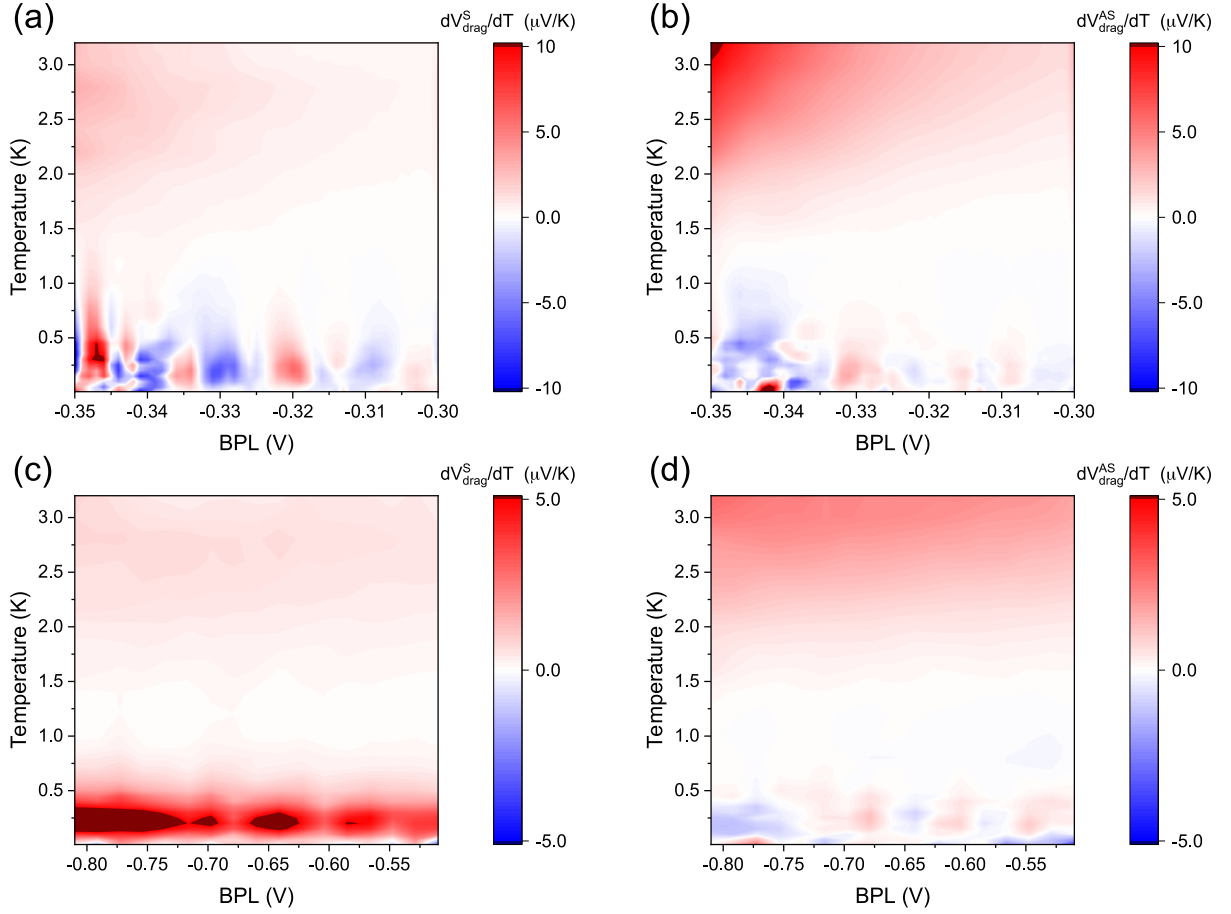

Fig. S13. BPL gate-temperature drag voltage derivative 2D plot. (a), (b), BPL gate-temperature 2D plot of drag voltage derivative with respect to temperature at TPL=-0.735V of (a) the symmetric component and (b) the antisymmetric component. (c), (d), BPL gate-temperature 2D plot of drag voltage derivative with respect to temperature at BPL=-0.32V of (c) the symmetric component and (d) the antisymmetric component. The first derivative sign changes with the wire subband changes which are consistent with the fitting exponent sign changes in Fig. 5. The tuning points  $T^*$  s between the two temperature regimes appear as a white band in the derivative 2D plot. Compared to the dependence of the antisymmetric component's tuning point  $T_{AS}^*$  on both the drag and drive wire electron density, the symmetric component's tuning point  $T_S^*$  has negligible dependence on the drive wire electron density, stressing the different mechanisms behind the origin of these two components.

### VIII. STRIPES WITH SLOPE

As shown in Fig. S14(a), the top (drive) wire subband positions start to shift to the positive side once the bottom PL gate is lower than -0.3V, compared with the consistent subband positions of the bottom (drag) wire shown in Fig. S14(b). To further show the sloped stripes in Fig. 2, the drive current 2D map is shown in Fig. S14(c) and the differential conductance of the drive wire 2D map is shown in Fig. S14(d). In both Fig. S14(c) and Fig. S14(d), the sloped stripes are clear and consistent with that the top wire subband positions shift to the positive side as the bottom wire gets closed to pinch off, which confirms they are the constant density lines of the top wire.

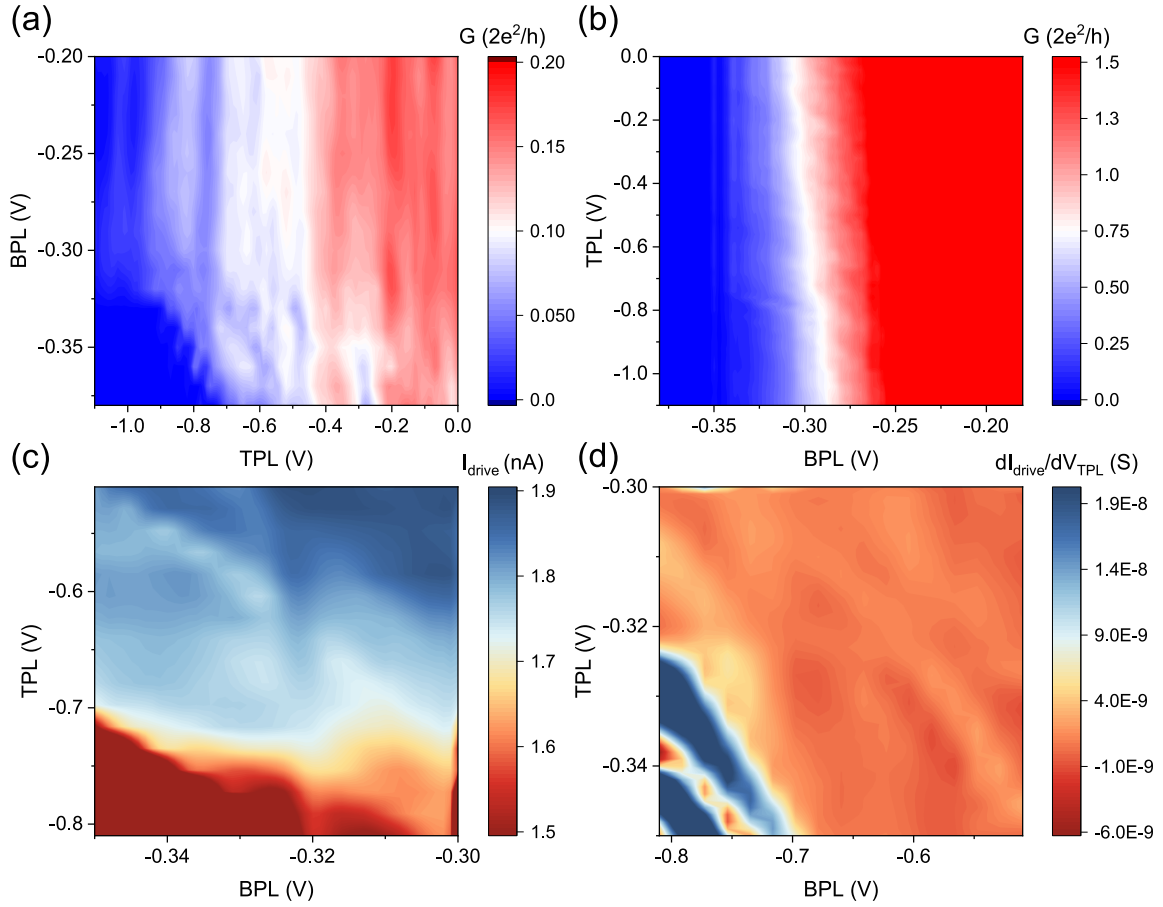

Fig. S14. Stripes with slope. (a), (b), The conductance 2D map as a function of both TPL and BPL gate positions for (a) the top wire, and (b) the bottom wire. The top wire subband positions shift as the bottom wire subband changes. (c), The drive current 2D map as a function of the TPL(drive) and BPL(drag) gate positions. (d), The differential conductance of the drive wire for (c). The stripes with slope are clear in both (c) and (d), which is related to the BPL gate dependent top wire subband positions.

## IX. CALCULATION OF THE ERROR BARS OF THE FITTING PARAMETERS

The error bars of exponential dependence of the drag magnitude on  $k_f d$ , presented in the inset of Fig.4(f), were determined using a bootstrap Monte Carlo method. Assuming a normal distribution with the reported value as the mean and the error as the standard deviation, we randomly generated a new series of points. We generated 10000 such datasets and then fitted the linear equation  $I = B * V_{BPL} + I_0$  to each of these datasets. The standard deviation of the calculated exponents  $A$  of all the datasets  $\Delta S$  was then used as the error on the slope. Therefore, the error of the ratio  $r_{INT} = \frac{B_{AS}}{B_S}$  will be calculated to be  $\Delta r_{INT} = r_{INT} * \sqrt{(\frac{\Delta B_{AS}}{B_{AS}})^2 + (\frac{\Delta B_S}{B_S})^2}$ .

- 
- [1] D. Laroche, G. Gervais, M. P. Lilly, and J. L. Reno, Positive and negative Coulomb drag in vertically integrated one-dimensional quantum wires, *Nature Nanotechnology* **6**, 793 (2011).
  - [2] P. Debray, V. Zverev, O. Raichev, R. Klesse, P. Vasilopoulos, and R. S. Newrock, Experimental studies of Coulomb drag between ballistic quantum wires, *Journal of Physics: Condensed Matter* **13**, 3389 (2001).
  - [3] M. Yamamoto, M. Stopa, Y. Tokura, Y. Hirayama, and S. Tarucha, Negative Coulomb Drag in a One-Dimensional Wire, *Science* **313**, 204 (2006).
  - [4] D. Laroche, G. Gervais, M. P. Lilly, and J. L. Reno, 1D-1D Coulomb Drag Signature of a Luttinger Liquid, *Science* **343**, 631 (2014).

- [5] S. M. Tabatabaei, D. Sánchez, A. L. Yeyati, and R. Sánchez, Andreev-coulomb drag in coupled quantum dots, *Physical Review Letters* **125**, 247701 (2020).
- [6] L. Anderson, A. Cheng, T. Taniguchi, K. Watanabe, and P. Kim, Coulomb drag between a carbon nanotube and monolayer graphene, *Physical Review Letters* **127**, 257701 (2021).
- [7] Y. Tang, J.-W. Lee, A. Tylan-Tyler, H. Lee, M. Tomczyk, M. Huang, C.-B. Eom, P. Irvin, and J. Levy, Frictional drag between superconducting  $\text{LaAlO}_3/\text{SrTiO}_3$  nanowires, *Semiconductor Science and Technology* **35**, 09LT01 (2020).
- [8] R. Makaju, H. Kassar, S. M. Daloglu, A. Huynh, D. Laroche, A. Levchenko, and S. J. Addamane, Nonreciprocal coulomb drag between quantum wires in the quasi-one-dimensional regime, *Phys. Rev. B* **109**, 085101 (2024).
